# Supplementary material for: Coordination Failure in Cooperative Offline MARL
Source: arXiv:2407.01343 source file (2024-07-01)
Supplement: Supplementary file 1 [file 99-appendix.tex]

\appendix

\section{Appendix / supplemental material}

Optionally include supplemental material (complete proofs, additional experiments and plots) in appendix.
All such materials \textbf{SHOULD be included in the main submission.}
